# Supplementary material for: Towards Cost-efficient Sampling Methods
Source: arXiv:1405.5756 source file (2014-05-22)
Supplement: Supplementary file 1 [file Supplementary_Materials.pdf]

**Supplementary Materials: Main Codes (only for publishing online)**

```
%%%%%%%%%%%%%%%%%%%%%%%%%%%%%%
%The codes can be run in Matlab 7.0 and its above versions%
%Authors keep all the rights of these codes%%%%%%%%%
%%%%%%%%%%%%%%%%%%%%%%%%%%%%%%
%%%%%%%%%%%%%%%%%%%%%%%%%%%%%%%%%%%%%%%%%%%%%
%Here is the program of the ISRS (improved stratified random sampling) method (function)%
%%%%%%%%%%%%%%%%%%%%%%%%%%%%%%%%%%%%%%%%%%%%%
  function [a1,y]=isrs(a,n,x)
  a2=zeros(n);y2=0;d=zeros(1,n);
  for i=1:1:n
       if rand(1)<=x
           a2(i,i)=1;y2=y2+1;d(1,i)=sum(a(i,:));
       end
  end
  c=shouxun(d,y2);y=0;a1=zeros(n)
  for i=1:1:n
       if a(i,i)==1 && d(1,i)>=c && rand(1)<=0.8
           a1(i,i)=1;y=y+1;
       elseif a(i,i)==1 && d(1,i)<=c && rand(1)<=0.3
           a1(i,i)=1;y=y+1;
       end
  end

%%%%%%%%%%%%%%%%%%%%%%%%
%Here is the program of the shouxun (function)%
%%%%%%%%%%%%%%%%%%%%%%%%
  function c=shouxun(b1,y)
  d=max(b1);f=min(b1);e=d-f;
  for i=1:1:e
       d=d-2;h=0;
       for j=1:1:y
            if b1(j)>=d
               h=h+1;
            end
       end
       if h/n>=0.2
          break;
       end
  end
  c=d;
```

```
%%%%%%%%%%%%%%%%%%%%%%%%%%%%%%%%%%%%%%%%%%%%
%Here is the program of the ISBS(improved snowball sampling) method (function)%
%%%%%%%%%%%%%%%%%%%%%%%%%%%%%%%%%%%%%%%%%%%%
    function [a1,m,b4]=isnowball(a,n,x)
    a1=zeros(n,n);b4=0;
    b1=zeros(1,n);
    b2=zeros(1,n);
    for i=1:1:n
            b1(1,i)=i;
    end
    b=unidrnd(n);
    for i=1:1:n
            if sum(a(b,:))<2
                 b=unidrnd(n);
            else break;
            end
    end
    m=0;b2(1,1)=b;b1(b1==b)=[];t1=1;
    while m<n*x
             if m+t1<=n*x
                  k=1;
                  while b2(1,k)>0
                           a1(b2(1,k),b2(1,k))=1;m=m+1;b1(b1==b2(1,k))=[];b4=[b4,b2(1,k)];
                           k=k+1;
                  end
              elseif m+t1>n*x
                    [a1,m,b4]=isnowball2(a,a1,b2,b3,n,x,t1,m,b4);
              end
              [b3,t]=isnowball1(a,b1,b2,n);
              b2=b3;t1=t;
              if t<2
                   [b3,b2,b1,t,t1,m,b4]=isnowball3(a,b1,n,m,b4);
              end
    end

%%%%%%%%%%%%%%%%%%%%%%%%%
%Here is the program of the isnowball1 (function)%
%%%%%%%%%%%%%%%%%%%%%%%%%
    function [b4,j]=isnowball1(a,b1,b2,n)
    k=1;b3=zeros(1,n);t=0;b4=zeros(1,n);
    while b2(1,k)>0
       for i=1:1:n
```

```
            if a(b2(1,k),i)==1 & ismember(i,b1)>0 & ismember(i,b3)==0 & ismember(i,b2)==0
                t=t+1;b3(1,t)=i;
            end
        end
        k=k+1;
    end
    c1=zeros(1,t);
    for i=1:1:t
        c1(1,i)=sum(a(b3(1,i),:));
    end
    c=shouxun(c1,t);j=0;
    for i=1:1:t
          if c1(1,i)>=c
              j=j+1;b4(1,j)=b3(1,i);
          end
    end

%%%%%%%%%%%%%%%%%%%%%%%%%%%%%%%%
%Here is the program of the isnowball2 (function)%
%%%%%%%%%%%%%%%%%%%%%%%%%%%%%%%%%%
    function [a1,m,b4]=isnowball2(a,a1,b2,b3,n,x,t1,m,b4)
    e=0;c=zeros(1,t1);
    for i=1:1:t1
          c(1,i)=sum(a(b2(1,i),:));
    end
    while m+e<n*x
       d=max(c);
       for i=1:1:t1
            if c(1,i)==d
                 a1(b2(1,i),b2(1,i))=1;e=e+1;
                 c(i)=[];b4=[b4,b2(1,i)];t1=t1-1;break;
             end
       end
    end
    m=m+e;

%%%%%%%%%%%%%%%%%%%%%%%%%%%%%%%%
%Here is the program of the isnowball3 (function)%
%%%%%%%%%%%%%%%%%%%%%%%%%%%%%%%%
    function [b5,b2,b1,j,t1,m,b4]=isnowball3(a,b1,n,m,b4)
    b=unidrnd(n);
    while sum(a(b,:))<2 | ismember(b,b1)==0
```

```
        b=unidrnd(n);
    end
    b2=zeros(1,n);
    b2(1,1)=b;t=0;b3=zeros(1,n);
    for i=1:1:n
        if a(b,i)==1
            t=t+1;b3(1,t)=i;
        end
    end
    b5=zeros(1,n);
    c1=zeros(1,t);
    for i=1:1:t
      c1(1,i)=sum(a(b3(1,i),:));
    end
    c=shouxun(c1,t);j=0;t1=1;
    for i=1:1:t
        if c1(1,i)>c
            j=j+1;b5(1,j)=b3(1,i);
        end
    end

%%%%%%%%%%%%%%%%%%%%%%%%%%%%%%%%%%%%%%%%%%%%%%%%%%%%%%%%%%%%%%%%%%%%%%%%%%
%Here is the program of the ES(edge sampling) method (function)%
%%%%%%%%%%%%%%%%%%%%%%%%%%%%%%%%%%%%%%%%%%%%%%%%%%%%%%%%%%%%%%%%%%%%%%%%%%
    function a1=es(a,n,x)
    a1=a;
    for i=1:1:n
          for j=1:1:i-1
                if a(i,j)==1 & rand(1)>=x
                      a1(i,j)=0;a1(j,i)=0;
                end
          end
    end

%%%%%%%%%%%%%%%%%%%%%%%%%%%%%%%%%%%%%%%%%%%%%%%%%%%%%%%%%%%%%%%%%%%%%%%%%%
%Here is the program of the NS(node sampling) method (function)%
%%%%%%%%%%%%%%%%%%%%%%%%%%%%%%%%%%%%%%%%%%%%%%%%%%%%%%%%%%%%%%%%%%%%%%%%%%
    function [a1,y]=ns(a,n,x)
    a1=eye(n);y=n;
    for i=1:1:n
          if rand(1)>=x
                a1(i,i)=0;y=y-1;
```

```
            end
      end

%%%%%%%%%%%%%%%%%%%%%%%%%%%%%%%%%%%%%%%%%%%
%Here is the program of the SRS(stratified random sampling) method (function)%
%%%%%%%%%%%%%%%%%%%%%%%%%%%%%%%%%%%%%%%%%%%
      function [a1,y]=srs(a,n,x)
      a2=zeros(n);y2=0;d=zeros(1,n);
      for i=1:1:n
            if rand(1)<=x
                  a2(i,i)=1;y2=y2+1;d(1,i)=sum(a(i,:));
            end
      end
      c=shouxun(d,y2);y=0;a1=zeros(n)
      for i=1:1:n
            if a(i,i)==1 && d(1,i)>=c && rand(1)<=0.2
                  a1(i,i)=1;y=y+1;
            elseif a(i,i)==1 && d(1,i)<=c && rand(1)<=0.8
                  a1(i,i)=1;y=y+1;
            end
      end

%%%%%%%%%%%%%%%%%%%%%%%%%%%%%%%%%%%%%%%%%%%
%Here is the program of the SBS(snowball sampling) method (function)%
%%%%%%%%%%%%%%%%%%%%%%%%%%%%%%%%%%%%%%%%%%%
      function [a1,m]=snowball(a,n,x)
      a1=zeros(n,n);b4=0;
      b1=zeros(1,n);
      b2=zeros(1,n);
      for i=1:1:n
            b1(1,i)=i;
      end
      b=unidrnd(n);
      for i=1:1:n
            if sum(a(b,:))==0
                 b=unidrnd(n);
            else break;
            end
      end
      m=1;b2(1,1)=b;b1(b1==b)=[];b4=[b4,b];
      while m<n*x
             [b3,t]=snowball1(a,b1,b2,n);
```

```
            if t==0
                  [b3,b2,b1,t,m,b4]=snowball3(a,b1,n,m,b4);
            end
            if m+t<=n*x
                  k=1;
                  while b2(1,k)>0
                              a1(b2(1,k),:)=a(b2(1,k),:);
                              a1(:,b2(1,k))=a(:,b2(1,k));m=m+sum(a(b2(1,k),:));
                              for i=1:1:n
                                    if a(b2(1,k),i)==1 & ismember(i,b1)>0
                                            b1(b1==i)=[];b4=[b4,i];
                                    end
                              end
                              k=k+1;
                  end
              elseif m+t>n*x
                      [a1,m,b4]=snowball2(a,a1,b1,b2,b3,n,x,t,m,b4);
              end
              b2=b3;
     end

%%%%%%%%%%%%%%%%%%%%%%%%%%
%Here is the program of the snowball1 (function)%
%%%%%%%%%%%%%%%%%%%%%%%%%%
     function [b3,t]=snowball1(a,b1,b2,n)
     k=1;b3=zeros(1,n);t=0;
     while b2(1,k)>0
         for i=1:1:n
               if a(b2(1,k),i)==1 & ismember(i,b1)>0 & ismember(i,b3)==0 & ismember(i,b2)==0
                     t=t+1;b3(1,t)=i;
               end
           end
           k=k+1;
     end

%%%%%%%%%%%%%%%%%%%%%%%%%%
%Here is the program of the snowball2 (function)%
%%%%%%%%%%%%%%%%%%%%%%%%%%
     function [a1,m,b4]=snowball2(a,a1,b1,b2,b3,n,x,t,m,b4)
     e=0;
     while m+e<n*x
         y=unidrnd(t);k=1;
```

```
        while b2(1,k)>0
            if a(b2(1,k),b3(1,y))==1
                a1(b2(1,k),b3(1,y))=1;a1(b3(1,y),b2(1,k))=1;e=e+1;
                b3(b3==b3(1,y))=[];b4=[b4,b3(1,y)];t=t-1;break;
            end
            k=k+1;
        end
    end
    m=m+e;

%%%%%%%%%%%%%%%%%%%%%%%%%%
%Here is the program of the snowball3 (function)%
%%%%%%%%%%%%%%%%%%%%%%%%%%
    function [b3,b2,b1,t,m,b4]=snowball3(a,b1,n,m,b4)
    b=unidrnd(n);
    while sum(a(b,:))==0 & ismember(b,b1)==0
        b=unidrnd(n);
    end
    b2=zeros(1,n);
    m=m+1;b2(1,1)=b;b1(b1==b)=[];t=0;b3=zeros(1,n);b4=[b4,b];
    for i=1:1:n
        if a(b,i)==1
            t=t+1;b3(1,t)=i;
        end
    end

%%%%%%%%%%%%%%%%%%%%%%%%%%%%%%%%%%%%%%%%
%Here is the program of the RWS(random walk sampling) method (function)%
%%%%%%%%%%%%%%%%%%%%%%%%%%%%%%%%%%%%%%%%
    function [a1,y,b4]=rws(a,n,x)
    a1=zeros(n,n);y=1;b4=0;
    b=unidrnd(n);
    b1=zeros(1,n);
    for i=1:1:n
         b1(1,i)=i;
    end
    while sum(a(b,:))==0
            b=unidrnd(n);
    end
    b1(b1==b)=[];c=sum(a(b,:));b4=[b4,b];a1(b,b)=1;
    while y<n*x
            d=unidrnd(c);
```

```
        j=0;
        for i=1:1:n
            if j==d
                i=i-1;break;
            elseif    a(b,i)==1 & ismember(i,b1)==1
                j=j+1;
            end
         end
         a1(i,i)=1;b1(b1==i)=[];b4=[b4,i];y=y+1;
         b=i;j=0;
         for i=1:1:n
              if a(b,i)==1 & ismember(i,b1)==1
                  j=j+1;
              end
         end
         c=j;
         if j==0
            b==unidrnd(n);t=0;
            for i=1:1:n
                if a(b,i)==1 & ismember(i,b1)==1
                    t=t+1;
                end
            end
            while t==0 | ismember(b,b1)==0
                    b=unidrnd(n);t=0;
                    for i=1:1:n
                        if a(b,i)==1 & ismember(i,b1)==1
                            t=t+1;
                        end
                    end
            end
            c=t;
            y=y+1;b1(b1==i)=[];b4=[b4,i];a1(b,b)=1;
         end
  end

%%%%%%%%%%%%%%%%%%%%%%%%%%%%%%%%%%%%%%%%%%%%%%%%%%%%%%%%%%%%%%%%%%%%%
%Here is the program of the fS(frontier sampling) method (function)%
%%%%%%%%%%%%%%%%%%%%%%%%%%%%%%%%%%%%%%%%%%%%%%%%%%%%%%%%%%%%%%%%%%%%%
  function [a1,t]=fs(a,n,x)
  a1=zeros(n,n);s=0;s1=0;n1=sum(sum(a));t=0;i=0;
  while i<n*0.05
```

```
            b=unidrnd(n);
            if sum(a(b,:))>0
                s=[s,b];s1=[s1,sum(a(b,:))];i=i+1;
                a1(b,b)=1;
            end
    end
    s(s==0)=[];s1(s1==0)=[];b1=s;
    k=size(s1,2);t=k;
    while t<=n*x
          b=rand(1);y=s1(1,1)/sum(s1);
              for i=1:1:k-1
                     if y>=b
                           [s,s1,a1,t,b1]=huandian(a,a1,s,s1,i,n,t,b1);break;
                     else y=y+s1(1,i+1)/sum(s1);
                     end
              end
    end

%%%%%%%%%%%%%%%%%%%%%%%%%%%%%%%
%Here is the program of the huandian (function)
%%%%%%%%%%%%%%%%%%%%%%%%%%%%%%%
    function [s,s1,a1,t,b1]=huandian(a,a1,s,s1,i,n,t,b1)
    f=0;
    for j=1:1:n
          if a(s(1,i),j)==1 & ismember(j,b1)==0
                f=f+1;
          end
    end
    b=unidrnd(f);k=0;
    for j=1:1:n
          if a(s(1,i),j)==1 & b==k & ismember(j,b1)==0
                a1(j,j)=1;s(1,i)=j;s1(1,i)=sum(a(j,:));t=t+1;b1=[b1,j];
                if sum(a(j,:))==0
                      b=unidrnd(n);
                      while sum(a(b,:))==0 | ismember(b,b1)==1
                                b=unidrnd(n);
                      end
                      s(1,i)=b;s1(1,i)=sum(a(b,:));t=t+1;
                      a1(b,b)=1;
                  end
          elseif a(s(1,i),j)==1 & ismember(j,b1)==0
                k=k+1;
```

```
    end
end
```
